# Supplementary material for: 4DAnyone: Create Anyone in 4D from a Casual Monocular Video
Source: arXiv:2608.20335 source file (2026-08-20)
Supplement: Supplementary file 1 [file supp.tex]

\documentclass[acmtog,nonacm]{acmart}

\input{preamble}

% TOG prefers author-name bibliography with square brackets.
\citestyle{acmauthoryear}

\begin{document}

\title{\papertitle}
\newcommand{\supplementaryversion}{}
\input{author_info}
\hypersetup{%
  pdftitle={\papertitle: Supplementary Material},
  pdfauthor={\pdfauthors}}
\ccsdesc[500]{Computing methodologies~Multi-View \& 3D}
\keywords{multiview video generation, 4D human reconstruction}

\input{docs/supp}

\clearpage
\bibliographystyle{ACM-Reference-Format}
\bibliography{main}

\end{document}
